# Supplementary material for: Specification Mining for Smart Contracts with Trace Slicing and Predicate Abstraction
Source: arXiv:2403.13279 source file (2025-04-29)
Supplement: Supplementary file 1 [file Appendix.tex]

%!TEX root = ../main.tex
\section{The \gamechannel Source Code}\label{sec:source}

%	\begin{lrbox}{\mintedbox}
%		% coerce minted to produce a box, rather than a full width environment
%		\RecustomVerbatimEnvironment{Verbatim}{BVerbatim}{}

The following shows the simplified source code of \gamechannel.
The \texttt{constructor} function specifies the server address who administrates the application
\comment{check line numbers!}{(Lines 11--13)}.
To play the game, users create a game session by calling \texttt{createGame} (Lines 14--20).
Then, actual gambling process will continue and be managed on another high-throughput side
blockchain maintained by \dicether.
When approaching the end, \texttt{server} user will end the game by calling \texttt{serverEndGame}
(Lines 21--25).
If there are other reasons for terminating game,
the other game functions (Lines 26--74): \texttt{serverForceGameEnd},
\texttt{userCancelActiveGame}, \texttt{serverCancelActiveGame}, \texttt{serverEndGameConflict}, and
\texttt{userEndGameConflict}
can be used.

\begin{minted}[texcomments,fontsize=\footnotesize,breaklines,linenos]{solidity}
contract GameChannel{
  enum GameStatus {
    ENDED, ACTIVE, USER_INITIATED_END, SERVER_INITIATED_END
  }

  struct Game {
    GameStatus status; uint128 stake; uint32 roundId; uint endInitiatedTime;
  }

  uint public gameIdCntr = 0;  /// @dev Game id counter.
  address public server;
  mapping (uint => Game) public gameIdGame;
  mapping (address => uint) public userGameId;
  modifier onlyServer() { require(msg.sender == server); _; }

  constructor(address _server) public{
    server = _server;
  }

  function createGame() public payable{
    uint gameId = gameIdCntr++;
    userGameId[msg.sender] = gameId;
    Game storage newGame = gameIdGame[gameId];
    require(msg.value>0);
    newGame.stake = uint128(msg.value);
    newGame.status = GameStatus.ACTIVE;
  }

  function serverEndGame(uint _gameId) public onlyServer{
    Game storage game = gameIdGame[_gameId];
    require(game.status == GameStatus.ACTIVE, "inv status");
    game.status = GameStatus.ENDED;
  }

  function serverForceGameEnd(uint _gameId) public onlyServer{
    Game storage game = gameIdGame[_gameId];
    require(game.status == GameStatus.SERVER_INITIATED_END, "inv status");
    game.status = GameStatus.ENDED;
  }

  function userCancelActiveGame(uint _gameId) public{
    require(_gameId == userGameId[msg.sender]);
    Game storage game = gameIdGame[_gameId];
    if (game.status == GameStatus.ACTIVE) {
      game.status = GameStatus.USER_INITIATED_END;
      game.endInitiatedTime = block.timestamp;
    } else if (game.status == GameStatus.SERVER_INITIATED_END && game.roundId == 0) {
      game.status = GameStatus.ENDED;
    } else { revert();}
  }

  function serverCancelActiveGame(uint _gameId) public onlyServer{
    Game storage game = gameIdGame[_gameId];
    if (game.status == GameStatus.ACTIVE) {
      game.status = GameStatus.SERVER_INITIATED_END;
      game.endInitiatedTime = block.timestamp;
    } else if (game.status == GameStatus.USER_INITIATED_END && game.roundId == 0) {
      game.status = GameStatus.ENDED;
    } else { revert(); }
  }

  function serverEndGameConflict(uint32 _roundId, uint _gameId) public onlyServer{
    Game storage game = gameIdGame[_gameId];
    require(_roundId > 0, "inv roundId");
    if (game.status == GameStatus.USER_INITIATED_END && game.roundId == _roundId) {
      game.status = GameStatus.ENDED;
    } else if (game.status == GameStatus.ACTIVE || (game.status == GameStatus.USER_INITIATED_END &&
      game.roundId < _roundId)) {
      game.status = GameStatus.SERVER_INITIATED_END;
      game.endInitiatedTime = block.timestamp;
      game.roundId = _roundId;
    } else { revert(); }
  }

  function userEndGameConflict(uint32 _roundId, uint _gameId) public{
    require(_gameId == userGameId[msg.sender]);
    Game storage game = gameIdGame[_gameId];
    require(_roundId > 0, "inv roundId");
    if (game.status == GameStatus.SERVER_INITIATED_END && game.roundId == _roundId) {
      game.status = GameStatus.ENDED;
    } else if (game.status == GameStatus.ACTIVE || (game.status == GameStatus.SERVER_INITIATED_END
    && game.roundId < _roundId)) {
      game.status = GameStatus.USER_INITIATED_END;
      game.endInitiatedTime = block.timestamp;
      game.roundId = _roundId;
    } else { revert();}
  }
}
\end{minted}
%\end{lrbox}
% \resizebox{\textwidth}{!}{\usebox{\mintedbox}}
%	\caption{Simplified code for \gamechannel.}
%	\label{fig:dicether-code}
%\end{figure}

\begin{table*}[t]\centering
	\caption{The contract evolution of Dicether.}\label{tab:instances}
	\small
	\resizebox{\textwidth}{!}{
	\begin{tabular}{lcrrrrr}\toprule
	Id &Address &Commit &Solidity version &Deployment date &Last tx date &Total transactions \\\midrule
	1 & 0xc95d227a1cf92b6fd156265aa8a3ca7c7de0f28e & \href{https://github.com/dicether/contracts/commit/e69d8f537306a5035497660d44928ec0d1fb771c}{e69d8f53}&0.4.18 &Mar-31-2018 &May-29-2018 &830 \\
	2 &0xbf8b9092e809de87932b28ffaa00d520b04359aa & \href{https://github.com/dicether/contracts/commit/944417a4064806b8c32f0a3574d900a88b78a6e6}{944417a4}&0.4.24 &May-29-2018 &Aug-25-2018 &687 \\
	3 &0x3e07881993c7542a6da9025550b54331474b21dd & \href{https://github.com/dicether/contracts/commit/e864213051b4274481a00582a6ef96ced07ec171}{e8642130}&0.4.24 &Aug-25-2018 &Sep-06-2018 &147 \\
	4 &0xeb6f4ec38a347110941e86e691c2ca03e271df3b & \href{https://github.com/dicether/contracts/commit/ce3e3fefcee68d7bc7374dc6e9ca4b06f1283f1a}{ce3e3fef} & 0.4.24 &Sep-06-2018 &Oct-25-2018 &2,294 \\
	5 &0x9919d97e50397b7483e9ea61e027e4c4419c8171 & \href{https://github.com/dicether/contracts/commit/d40155728b4d5623e8a19a6a32818b676ea67ca7}{d4015572} &0.4.24 &Sep-28-2018 &Feb-14-2019 &4,720 \\
	6 &0x7e0178e1720e8b3a52086a23187947f35b6f3fc4 & \href{https://github.com/dicether/contracts/commit/2d96213ca8bb8bbdf57c6d684e5a7a6a53e8b102}{2d96213c} &0.5.0 &Feb-06-2019 &Mar-31-2019 &2,893 \\
	7 &0xaec1f783b29aab2727d7c374aa55483fe299fefa & \href{https://github.com/dicether/contracts/commit/91deaf6e06141f6bbae10b21e5b0ea6bedd9a16c}{91deaf6e}&0.5.0 &Mar-31-2019 &Mar-12-2022 &11,551 \\
	8 &0xa867bF8447eC6f614EA996057e3D769b76a8aa0e & \href{https://github.com/dicether/contracts/commit/dbcd3ac095ba0f315c5e9ba78928a59848256ec2}{dbcd3ac0} &0.8.11 &Mar-13-2022 & Jan-14-2024 &1,974 \\
	\bottomrule
	\end{tabular}
}
\end{table*}

\begin{figure}[t]
	\includegraphics[width=.8\columnwidth]{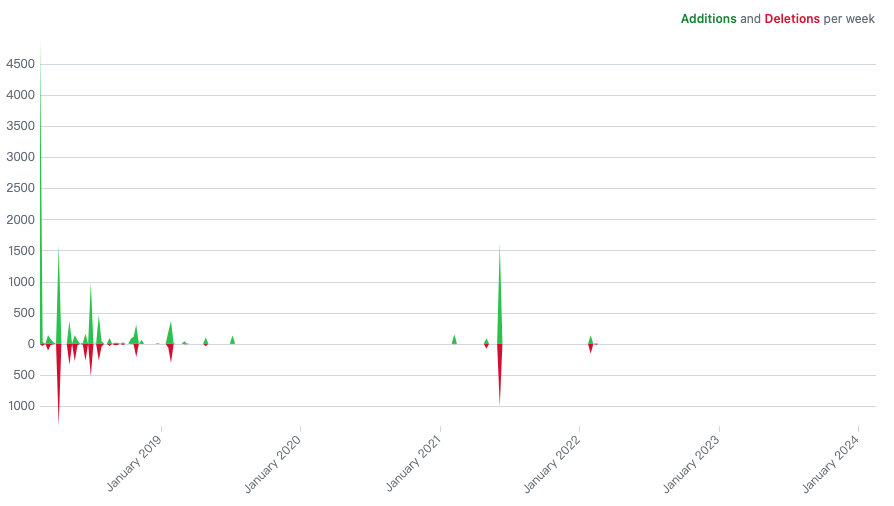}
	\caption{The git addition and deletion activities of Dicether.}\label{fig:git}
\end{figure}

\begin{figure*}[t]
	\includegraphics[width=\textwidth]{figure/gamechannel/0xC95D227a1CF92b6FD156265AA8A3cA7c7DE0F28e/GameChannel/smcon.pdf}
	\caption{Dicether (0xc95d227a1cf92b6fd156265aa8a3ca7c7de0f28e).}
	\label{fig:0xc9}
\end{figure*}

\begin{figure*}
	\includegraphics[width=\textwidth]{figure/gamechannel/0xeb6f4ec38a347110941e86e691c2ca03e271df3b/GameChannel/smcon.pdf}
	\caption{0xeb6f4ec38a347110941e86e691c2ca03e271df3b}
\end{figure*}

\begin{figure*}[t]
	\includegraphics[width=\textwidth]{figure/gamechannel/0xaec1f783b29aab2727d7c374aa55483fe299fefa/GameChannel/smcon.pdf}
	\caption{Dicether (0xaec1f783b29aab2727d7c374aa55483fe299fefa).}
	\label{fig:0xae}
\end{figure*}

\begin{figure*}
	\includegraphics[width=\textwidth]{figure/gamechannel/0xa867bF8447eC6f614EA996057e3D769b76a8aa0e/GameChannel/smcon.pdf}
	\caption{0xa867bF8447eC6f614EA996057e3D769b76a8aa0e}
\end{figure*}
